# Supplementary material for: Long-timescale predictions from short-trajectory data: A benchmark analysis of the trp-cage miniprotein
Source: arXiv:2009.04034 source file (2020-09-08)
Supplement: Supplementary file 2 [file suppaux.tex]

\begin{filecontents}{supp.aux}
\relax 
\citation{achemso-control}
\providecommand{\mciteSetMaxWidth}[3]{\relax}
\providecommand{\mciteSetMaxCount}[3]{\relax}
\bibstyle{achemso}
\@writefile{toc}{\contentsline {section}{\numberline {A}Backward-in-time inner products}{1}}
\newlabel{secn:innerproductderivation}{{A}{1}}
\newlabel{eq:fbpath}{{S3}{2}}
\citation{vanden2006transition}
\citation{vanden2006transition}
\@writefile{toc}{\contentsline {section}{\numberline {B}A formula for the reactive current}{3}}
\newlabel{eqn:JAB}{{S9}{3}}
\newlabel{eqn:eqCurrent}{{S11}{3}}
\newlabel{eqn:JABgrad}{{S12}{4}}
\newlabel{eqn::1}{{S15}{4}}
\newlabel{eq:estimator_JABSup0}{{S16}{5}}
\newlabel{eq:estimator_JABSup}{{S17}{5}}
\@writefile{toc}{\contentsline {section}{\numberline {C}Reactive current on a CV space}{5}}
\newlabel{secn:cvcurrent}{{C}{5}}
\bibstyle{achemso}
\bibdata{acs-supp,references,trp_cage_bib,dga_paper}
\newlabel{eqn:def1}{{S18}{6}}
\bibcite{vanden2006transition}{{1}{2006}{{Vanden-Eijnden}}{{}}}
\mciteSetMaxCount{main}{bibitem}{1}
\mciteSetMaxCount{main}{subitem}{1}
\mciteSetMaxWidth{main}{bibitem}{385020}
\mciteSetMaxWidth{main}{subitem}{0}
\@writefile{toc}{\contentsline {section}{References}{7}}
\@writefile{lof}{\contentsline {figure}{\numberline {S1}{\ignorespaces  EMUS asymptotic variance for REUS PMFs.\relax }}{8}}
\providecommand*\caption@xref[2]{\@setref\relax\@undefined{#1}}
\newlabel{fig:USAvars}{{S1}{8}}
\@writefile{lof}{\contentsline {figure}{\numberline {S2}{\ignorespaces  REUS PMFs.\relax }}{9}}
\newlabel{fig:REUS}{{S2}{9}}
\@writefile{lof}{\contentsline {figure}{\numberline {S3}{\ignorespaces  Difference between DGA with the modified distance basis set without the $\alpha $ helix resampling and REUS.\relax }}{10}}
\newlabel{fig:USminusDGAInitialSampling}{{S3}{10}}
\@writefile{lof}{\contentsline {figure}{\numberline {S4}{\ignorespaces  Difference between the PMF from DGA with the distance indicator basis set and the PMF from REUS.\relax }}{11}}
\newlabel{fig:USminusInd}{{S4}{11}}
\@writefile{lof}{\contentsline {figure}{\numberline {S5}{\ignorespaces  Difference between the PMF from DGA with the TICA indicator basis set and the PMF from REUS.\relax }}{12}}
\newlabel{fig:USminusTICA}{{S5}{12}}
\@writefile{lof}{\contentsline {figure}{\numberline {S6}{\ignorespaces  Difference between the PMF from DGA with the modified distance basis set and the PMF from REUS.\relax }}{13}}
\newlabel{fig:USminusSmooth}{{S6}{13}}
\@writefile{lof}{\contentsline {figure}{\numberline {S7}{\ignorespaces  DGA backward committors. Left, middle, and right columns are computed with the modified distance, distance indicator, and TICA indicator basis sets, respectively. Top, middle, and bottom rows are computed with lag times of 0.5, 2.5, and 7.5 ns, respectively.\relax }}{14}}
\newlabel{fig:backcomm}{{S7}{14}}
\end{filecontents}
